# Supplementary material for: Statistics of topological RNA structures
Source: arXiv:1606.06956 source file (2016-06-22)
Supplement: Supplementary file 1 [file Supplementary.pdf]

**Noname manuscript No.**
(will be inserted by the editor)

# Supplementary Material

**Thomas J. X. Li · Christian M. Reidys**

## 1 Four types of pseudoknots having genus one

- An *H-type pseudoknot* is a quintuple of the form $(K(i_1, j_1, k_1), K(i_2, j_2, k_2), S[i_1+1, i_2-k_2], S[i_2+1, j_1-1], S[j_1+k_1, j_2-1])$, where $S[i_1+1, i_2-k_2]$, $S[i_2+1, j_1-1]$ and $S[j_1+k_1, j_2-1]$ are secondary structures, $K(i_1, j_1, k_1)$ denotes a stack of length $k_1$ containing arcs $(i_1, j_1), (i_1-1, j_1+1), \ldots, (i_1-k_1+1, j_1+k_1-1)$, two arcs $(i_1, j_1)$ and $(i_2, j_2)$ form a crossing, i.e., $i_1 < i_2 < j_1 < j_2$,
- A *kissing hairpin* (K-type) is an octuple

  $$(K(i_1, j_1, k_1), K(i_2, j_2, k_2), K(i_3, j_3, k_3), S[i_1+1, i_2-k_2], S[i_2+1, j_1-1], S[j_1+k_1, i_3-k_3], S[i_3+1, j_2-1], S[j_2+k_2, j_3-1]),$$

  where $i_1 < i_2 < j_1 < i_3 < j_2 < j_3$,
- A *3-knot* (L-type) is an octuple

  $$(K(i_1, j_1, k_1), K(i_2, j_2, k_2), K(i_3, j_3, k_3), S[i_1+1, i_2-k_2], S[i_2+1, j_1-1], S[j_1+k_1, i_3-k_3], S[i_3+1, j_2-1], S[j_2+k_2, j_3-1]),$$

  where $i_1 < i_2 < i_3 < j_1 < j_2 < j_3$,
- A *4-knot* (M-type) consists of four stacks with arcs $(i_1, j_1), (i_2, j_2), (i_3, j_3), (i_4, j_4)$ and the secondary structures between them, where $i_1 < i_2 < i_3 < j_1 < i_4 < j_2 < j_3 < j_4$.

Thomas J. X. Li
Biocomplexity Institute of Virginia Tech
Blacksburg, VA 24061, USA
E-mail: thomasli@vbi.vt.edu

Christian M. Reidys
Biocomplexity Institute of Virginia Tech
Blacksburg, VA 24061, USA
E-mail: duckcr@vbi.vt.edu

## 2 Shape polynomials

$$\begin{aligned}
\mathbf{S}_1^H(x,y) &= x^2(1+x)\Big(x(x+2)+y\Big),\\
\mathbf{S}_2^H(x,y) &= x^4\,(1+x)^2\,\Big(17+143x+447x^2+637x^3+420x^4+105x^5\\
&\quad+\left(20x+36x^2+14x^3\right)y+(4+5x)y^2\Big),\\
\mathbf{S}_3^H(x,y) &= x^6\,(1+x)^3\,\Big(1259+21440x+138576x^2+465010x^3+909305x^4\\
&\quad+1078428x^5+765986x^6+300300x^7+50050x^8\\
&\quad+\left(204+2274x+9822x^2+20778x^3+22912x^4+12662x^5+2782x^6\right)y\\
&\quad+\left(182x+610x^2+632x^3+198x^4\right)y^2+\left(22+62x+42x^2\right)y^3\Big)\\
\mathbf{S}_4^H(x,y) &= x^8\,(1+x)^4\,\Big(202901+5340890x+55842220x^2+318030907x^3\\
&\quad+1122184501x^4+2616374172x^5+4158165268x^6+4540985673x^7\\
&\quad+3359729830x^8+1611463758x^9+452652200x^{10}+56581525x^{11}\\
&\quad+\big(20144+415454x+3309428x^2+13955648x^3+35189516x^4+55895722x^5\\
&\quad+56542892x^6+35406184x^7+12529060x^8+1918012x^9\big)y\\
&\quad+\big(2040+27744x+151922x^2+429062x^3+678378x^4+606026x^5\\
&\quad+286052x^6+55590x^7\big)y^2+\big(1632x+8196x^2+14624x^3\\
&\quad+10940x^4+2860x^5\big)y^3+\left(429x^3+916x^2+632x+140\right)y^4\Big)
\end{aligned}$$

## 3 Singularity analysis

Here we collect basic results from singularity analysis (Flajolet and Sedgewick, 2009). Let $f(x)=\sum_{n\geq 0} a_n\, x^n$ be a combinatorial generating function. A function $f(x)$ is $\Delta_\rho$ analytic at its dominant singularity $x=\rho$, if it is analytic in some domain $\Delta_\rho(\phi,d)=\{x \mid |x|<d, x\neq\rho,\ |\mathrm{Arg}(x-\rho)|>\phi\}$, for some $\phi, d$, where $d>|\rho|$ and $0<\phi<\frac{\pi}{2}$. We set

$$\left(f(x)=O\left(g(x)\right)\ \text{ as } x\to\rho\right)\iff\left(f(x)/g(x) \text{ is bounded as } x\to\rho\right),$$

Noting that for any $\gamma\in\mathbb{C}\setminus 0$,

$$[x^n]f(x)=\gamma^n[x^n]f\left(\frac{x}{\gamma}\right),$$

we can, without loss of generality, reduce our analysis to the case where $x=1$ is the unique dominant singularity. The following transfer-theorem allows us to derive the asymptotics of coefficients from the asymptotic expansion of its generating function around its dominant singularity.

**Theorem 1 (Flajolet and Sedgewick (2009), Theorem VI.3, pp. 390)** *Let $f(x)$ be a $\Delta_1$ analytic function at its unique dominant singularity $x = 1$. Let*

$$g(x) = (1-x)^{\alpha} \log^{\beta}\left(\frac{1}{1-x}\right), \quad \alpha, \beta \in \mathbb{R}.$$

*That is we have in the intersection of a neighborhood of* 1

$$f(x) = O(g(x)) \quad \text{for } x \to 1.$$

*Then we have*

$$[x^n]f(x) = O\left([x^n]g(x)\right).$$

**Theorem 2 (Flajolet and Sedgewick (2009))** *Suppose $f(x) = (1-x)^{-\alpha}$, $\alpha \in \mathbb{C} \setminus \mathbb{Z}_{\leq 0}$, then*

$$[x^n]f(x) \sim \frac{n^{\alpha-1}}{\Gamma(\alpha)}\left[1 + \frac{\alpha(\alpha-1)}{2n} + \frac{\alpha(\alpha-1)(\alpha-2)(3\alpha-1)}{24n^2} + \frac{\alpha^2(\alpha-1)^2(\alpha-2)(\alpha-3)}{48n^3} + O\left(\frac{1}{n^4}\right)\right].$$

We shall end this section by stating the following central limit theorem due to Bender (Bender, 1973):

**Theorem 3 (Bender (1973))** *Suppose we are given the bivariate generating function*

$$f(x,u) = \sum_{n,t\geq 0} f(n,t)\, x^n\, u^t,$$

*where $f(n,t) \geq 0$ and $f(n) = \sum_t f(n,t)$. Let $\mathbb{X}_n$ be a r.v. such that $\mathbb{P}(\mathbb{X}_n = t) = f(n,t)/f(n)$. Suppose*

$$[x^n]f(x,e^s) = c(s)\, n^{\alpha}\, \gamma(s)^{-n}\left(1 + O\left(\frac{1}{n}\right)\right),$$

*uniformly in $s$ in a neighborhood of 0, where $c(s)$ is continuous and nonzero near 0, $\alpha$ is a constant, and $\gamma(s)$ is analytic near 0.*

*Then there exists a pair $(\mu, \sigma)$ such that the normalized random variable*

$$\mathbb{X}_n^* = \frac{\mathbb{X}_n - \mu\, n}{\sqrt{n\,\sigma^2}},$$

*converges in distribution to a Gaussian variable with a speed of convergence $O(n^{-\frac{1}{2}})$. That is we have*

$$\lim_{n\to\infty} \mathbb{P}\left(\mathbb{X}_n^* < x\right) = \frac{1}{\sqrt{2\pi}} \int_{-\infty}^{x} e^{-\frac{1}{2}t^2} \mathrm{d}t,$$

*where $\mu$ and $\sigma^2$ are given by*

$$\mu = -\frac{\gamma'(0)}{\gamma(0)} \quad \text{and} \quad \sigma^2 = \left(\frac{\gamma'(0)}{\gamma(0)}\right)^2 - \frac{\gamma''(0)}{\gamma(0)}.$$

## References

E.A. Bender. Central and local limit theorems applied to asymptotic enumeration. *J. Combin. Theory A*, 15:91–111, 1973.

P. Flajolet and R. Sedgewick. *Analytic Combinatorics.* Cambridge University Press New York, 2009.
